# Supplementary material for: Microtubule Tracking in Electron Microscopy Volumes
Source: arXiv:2009.08371 source file (2020-09-17)
Supplement: Supplementary file 1 [file appendix.tex]

\appendix
\newpage
\section{Parameters}

\begin{table}
  \centering
  \begin{tabular}{llr}
    {\bf Operation} \hspace{5mm} & {\bf Size} & \hspace{3mm} {\bf Feature Maps} \\
    \hline
    \hline
    Conv      & (3,3,3) & 12 \\
    Conv (1)  & (3,3,3) & 12 \\
    MaxPool   & (1,3,3) & 12 \\
    Conv      & (3,3,3) & 60 \\
    Conv (2)  & (3,3,3) & 60 \\
    MaxPool   & (1,3,3) & 60 \\
    Conv      & (3,3,3) & 300 \\
    Conv (3)  & (3,3,3) & 300 \\
    MaxPool   & (1,3,3) & 300 \\
    Conv      & (3,3,3) & 1500 \\
    Conv      & (3,3,3) & 1500 \\
    TConv     & (1,3,3) & 300 \\
    Concat (3)& & 600 \\
    Conv      & (3,3,3) & 300 \\
    Conv      & (3,3,3) & 300 \\
    TConv     & (1,3,3) & 60 \\
    Concat (2)& & 120 \\
    Conv      & (3,3,3) & 60 \\
    Conv      & (3,3,3) & 60 \\
    TConv     & (1,3,3) & 12 \\
    Concat (1)& & 24 \\
    Conv      & (3,3,3) & 12 \\
    Conv      & (3,3,3) & 12 \\
    Conv      & (1,1,1) & 1/10$^*$ \\
    \hline
    \hline
  \end{tabular}
  \vspace{5mm}
  \caption{3D-UNet architecture used for all models. ``TConv'' denotes a
  transposed convolution, ``Concat (i)'' concatenates feature maps from ``Conv
  (i)''. The final convolution (denoted by $^*$) produces 1 or 10 feature maps
  for models NMS\_SM and NMS/CC\_GRAD, respectively.}
\end{table}

\begin{table}
  \centering
  \begin{tabular}{l r}
    {\bf Parameter} & {\bf Value} \\
      \hline
      \hline
      Input Shape & (32, 322, 322) \\
      \hline
      Loss & MSE  \\
      \hline
      Optimizer & Adam~\cite{kingma2014adam} \\
      \hline
      Learning Rate & 5E-05 \\
      \hline
      $\beta_1$ & 0.95 \\
      \hline
      $\beta_2$ & 0.999 \\
      \hline
      Iterations & 300,000 \\
      \hline
      \hline
  \end{tabular}
  \hspace{3mm}
  \begin{tabular}{llr}
    {\bf Augmentation} & {\bf Parameter} & {\bf Value} \\
    \hline
    \hline
    Elastic   & control point spacing & (4,40,40) \\
              & jitter sigma          & (0, 2, 2) \\
              & subsample             & 8 \\
    \hline
    Rotation  & axis                  & z \\
              & angle                 & in $[0,\frac{\pi}{2}]$ \\
    \hline
    Section Defects & slip probability & 0.05 \\
              & shift probability     & 0.05 \\
              & max misalign          & 10 \\
    \hline
    Mirror    & n/a & \\
    \hline
    Transpose & axes & x, y \\
    \hline
    Intensity & scale                 & in $[0.9, 1.1]$ \\
              & shift                 & in $[-0.1, 0.1]$ \\
    \hline
    \hline
  \end{tabular}
  \vspace{5mm}
  %\caption{Training parameters used for all models. Augmentations were
  %performed using the gunpowder
  %library (\url{http://funkey.science/gunpowder}), see online
  %documentation for details.}
  \caption{Training parameters used for all models. Augmentations were
  performed using our augmentation library (\url{http://funkey.science/gunpowder}), see
  online documentation for details.}
\end{table}

\begin{table}
    \centering
\begin{tabular}{l r r r r r r r r}
  \bf Model  & \hspace{2mm} $\boldsymbol{\theta_S}$  & $\boldsymbol{\theta_P}$ & $\boldsymbol{\theta_D}$ & $\boldsymbol{\theta_E}$ & $\boldsymbol{\theta_C}$ & $\boldsymbol{\theta_d}$ & \hspace{2mm} \bf Block Size $\boldsymbol{b}$& \hspace{2mm} \bf Context Size $\boldsymbol{\overline{b}}$\\
    \hline
    \hline
    NMS\_GRAD  & 180 & -80 & 0 & 12 & 14 & 90  & (30, 250, 250) & (50,450,450)\\
    \hline
    CC\_GRAD   & 200  & -70 & 0 & 14 & 14 & 120 & (30, 250, 250) & (50,450,450)\\
    \hline
    NMS\_SM    & 180  & -70 & 0 & 14 & 16 & 120 & (30, 250, 250) & (50,450,450)\\
    \hline
    NMS\_RFC    & 180  & -90 & 0 & 12 & 14 & 90 & (30, 250, 250) & (50,450,450)\\
    \hline
    Baseline   & 60  & -100 & 0 & 12 & 10 & 140 & (30, 250, 250) & (50,450,450)\\
    \hline
    \hline
\end{tabular}
  \vspace{5mm}
    \caption{ILP validation best parameters for all considered models.}
\end{table}
